# Supplementary material for: Deterministic Sub-exponential Algorithm for Discounted-sum Games with Unary Weights
Source: arXiv:2405.02479 source file (2024-05-20)
Supplement: Supplementary file 1 [file appendix.tex]

\section{Proofs of \Cref{section: polynomials}}
